# Supplementary material for: Improved Variational Autoencoders for Text Modeling using Dilated Convolutions
Source: arXiv:1702.08139 source file (2017-06-18)
Supplement: Supplementary file 1 [file appendix.pdf]

|                      |                                                                                                                                                   |
|----------------------|---------------------------------------------------------------------------------------------------------------------------------------------------|
| <b>Society</b>       | do you think there is a god ?                                                                                                                     |
| <b>Science</b>       | how many orbitals are there in outer space ? how many orbitals are there in the solar system ?                                                    |
| <b>Health</b>        | what is the difference between _UNK and _UNK                                                                                                      |
| <b>Education</b>     | what is the difference between a computer and a _UNK ?                                                                                            |
| <b>Computers</b>     | how can i make flash mp3 files ? i want to know how to make a flash video so i can upload it to my mp3 player ?                                   |
| <b>Sports</b>        | who is the best soccer player in the world ?                                                                                                      |
| <b>Business</b>      | what is the best way to make money online ?                                                                                                       |
| <b>Music</b>         | who is the best artist of all time ?                                                                                                              |
| <b>Relationships</b> | how do i know if a guy likes me ?                                                                                                                 |
| <b>Politics</b>      | what do you think about Iran ?                                                                                                                    |
| <b>Society</b>       | what is the meaning of life ?                                                                                                                     |
| <b>Science</b>       | what is the difference between kinetic energy and heat ?                                                                                          |
| <b>Health</b>        | what is the best way to get rid of migraine headaches ?                                                                                           |
| <b>Education</b>     | what is the best way to study for a good future ?                                                                                                 |
| <b>Computers</b>     | what is the best way to install windows xp home edition ?                                                                                         |
| <b>Sports</b>        | who do you think will win the super bowl this year ?                                                                                              |
| <b>Business</b>      | i would like to know what is the best way to get a good paying job ?                                                                              |
| <b>Entertainment</b> | what do you think is the best movie ever ?                                                                                                        |
| <b>Relationships</b> | what is the best way to get over a broken heart ?                                                                                                 |
| <b>Politics</b>      | what do you think about the war in iraq ?                                                                                                         |
| <b>Society</b>       | what would you do if you had a million dollars ?                                                                                                  |
| <b>Mathematics</b>   | i need help with this math problem !                                                                                                              |
| <b>Health</b>        | what is the best way to lose weight ?                                                                                                             |
| <b>Education</b>     | what is the best college in the world ?                                                                                                           |
| <b>Computers</b>     | what is the best way to get a new computer ?                                                                                                      |
| <b>Sports</b>        | who should i start ?                                                                                                                              |
| <b>Business</b>      | what is the best way to get a good paying job ?                                                                                                   |
| <b>Entertainment</b> | who do you think is the hottest guy in the world ?                                                                                                |
| <b>Relationships</b> | what should i do ?                                                                                                                                |
| <b>Politics</b>      | who do you think will be the next president of the united states ?                                                                                |
| <b>Society</b>       | do you believe in ghosts ?                                                                                                                        |
| <b>Science</b>       | why is the sky blue ?                                                                                                                             |
| <b>Health</b>        | what is the best way to get rid of a cold ?                                                                                                       |
| <b>Reference</b>     | what do you do when you are bored ?                                                                                                               |
| <b>Computers</b>     | why ca n't i watch videos on my computer ? when i try to watch videos on my computer , i ca n't get it to work on my computer . can anyone help ? |
| <b>Sports</b>        | what do you think about the _UNK game ?                                                                                                           |
| <b>Business</b>      | what is the best way to get a job ?                                                                                                               |
| <b>Entertainment</b> | what is your favorite tv show ?                                                                                                                   |
| <b>Relationships</b> | how do you know when a guy likes you ?                                                                                                            |
| <b>Politics</b>      | what do you think about this ?                                                                                                                    |
| <b>Society</b>       | what is the name of the prophet muhammad ( pbuh ) ? i do n't know if he is a jew or not .                                                         |
| <b>Science</b>       | where can i find a picture of the _UNK _UNK _UNK _UNK ? i need to know the name of the insect that has the name of the whale .                    |
| <b>Health</b>        | what is the best way to get rid of a _UNK mole ?                                                                                                  |
| <b>Reference</b>     | does anyone know where i can find info on _UNK _UNK _UNK ? i am looking for the name of the _UNK _UNK .                                           |
| <b>Computers</b>     | does anyone know where i can find a picture of a friend 's cell phone ?                                                                           |
| <b>Sports</b>        | does anyone know where i can find a biography of _UNK ?                                                                                           |
| <b>Business</b>      | does anyone know where i can find a copy of the _UNK ?                                                                                            |
| <b>Music</b>         | does anyone know the name of the song and who sings it ?                                                                                          |
| <b>Relationship</b>  | how do i tell my boyfriend that i love him ? he is my best friend , but i dont know how to tell him . please help ! ! ! ! !                       |
| <b>Politics</b>      | where is osama bin laden ?                                                                                                                        |

Table 7: Text generated by conditioning on topic label.

|               |                                                                                                                                                                                                                                                                                                                      |
|---------------|----------------------------------------------------------------------------------------------------------------------------------------------------------------------------------------------------------------------------------------------------------------------------------------------------------------------|
| <b>1 star</b> | the food is good , but the service is terrible . i have been here three times and each time the service has been horrible . the last time we were there , we had to wait a long time for our food to come out . when we finally got our food , the food was cold and the service was terrible . i will not be back . |
| <b>2 star</b> | this place used to be one of my favorite places to eat in the area .                                                                                                                                                                                                                                                 |
| <b>3 star</b> | i 've been here a few times , and the food has always been good .                                                                                                                                                                                                                                                    |
| <b>4 star</b> | this is one of my favorite places to eat in the phoenix area . the food is good , and the service is friendly .                                                                                                                                                                                                      |
| <b>5 star</b> | my husband and i love this place . the food is great , the service is great , and the prices are reasonable .                                                                                                                                                                                                        |
| <b>1 star</b> | this is the worst hotel i have ever been to . the room was dirty , the bathroom was dirty , and the room was filthy .                                                                                                                                                                                                |
| <b>2 star</b> | my husband and i decided to try this place because we had heard good things about it so we decided to give it a try . the service was good , but the food was mediocre at best .                                                                                                                                     |
| <b>3 star</b> | we came here on a saturday night with a group of friends . we were seated right away and the service was great . the food was good , but not great . the service was good and the atmosphere was nice .                                                                                                              |
| <b>4 star</b> | my husband and i came here for brunch on a saturday night . the place was packed so we were able to sit outside on the patio . we had a great view of the bellagio fountains and had a great view of the bellagio fountains . we sat at the bar and had a great view of the bellagio fountains .                     |
| <b>5 star</b> | my husband and i came here for the first time last night and had a great time ! the food was amazing , the service was great , and the atmosphere was perfect . we will be back !                                                                                                                                    |
| <b>1 star</b> | this is the worst place i have ever been to . i will never go back .                                                                                                                                                                                                                                                 |
| <b>2 star</b> | i was very disappointed with the quality of the food and the service . i will not be returning .                                                                                                                                                                                                                     |
| <b>3 star</b> | this was my first time at this location and i have to say it was a good experience .                                                                                                                                                                                                                                 |
| <b>4 star</b> | this is a great place to grab a bite to eat with friends or family .                                                                                                                                                                                                                                                 |
| <b>5 star</b> | i am so happy to have found a great place to get my nails done .                                                                                                                                                                                                                                                     |
| <b>1 star</b> | my wife and i have been going to this restaurant for years . the last few times i have been , the service has been terrible . the last time we were there , we had to wait a long time for our food to arrive . the food is good , but not worth the wait .                                                          |
| <b>2 star</b> | the food is good , but the service leaves something to be desired .                                                                                                                                                                                                                                                  |
| <b>3 star</b> | i have been here a few times . the food is consistently good , and the service is good .                                                                                                                                                                                                                             |
| <b>4 star</b> | my wife and i have been here a few times . the food is consistently good , and the service is friendly .                                                                                                                                                                                                             |
| <b>5 star</b> | my husband and i have been coming here for years . the food is consistently good and the service is always great .                                                                                                                                                                                                   |
| <b>1 star</b> | the food was good but the service was terrible . we had to wait 45 minutes for our food to come out and it was cold . i will not be back .                                                                                                                                                                           |
| <b>2 star</b> | the food was good but the service was terrible . we had a party of 6 and the food took forever to come out . the food was good but not worth the price .                                                                                                                                                             |
| <b>3 star</b> | the food was good but the service was a little slow . we had to wait a while for our food and it was n't even busy .                                                                                                                                                                                                 |
| <b>4 star</b> | i have been here a few times and have never been disappointed . the food was great and the service was great . we will be back .                                                                                                                                                                                     |
| <b>5 star</b> | my husband and i have been here a few times and have never been disappointed . the food was great and the service was great . i will definitely be back !                                                                                                                                                            |
| <b>1 star</b> | if i could give this place zero stars i would . i do not recommend this place to anyone !                                                                                                                                                                                                                            |
| <b>2 star</b> | i do n't know what all the hype is about this place , but i do n't think i will be back .                                                                                                                                                                                                                            |
| <b>3 star</b> | i do n't know what all the hype is about this place , but i do n't think i 'll be back .                                                                                                                                                                                                                             |
| <b>4 star</b> | i 've been here a couple of times and have never been disappointed . the food is fresh , the service is friendly , and the prices are reasonable .                                                                                                                                                                   |
| <b>5 star</b> | this is the best ramen i 've ever had in my life , and i 've never had a bad meal here !                                                                                                                                                                                                                             |
| <b>1 star</b> | this is the worst company i have ever dealt with . they do n't know what they are doing .                                                                                                                                                                                                                            |
| <b>2 star</b> | this is the worst buffet i have ever been to in my life . the food was just ok , nothing to write home about .                                                                                                                                                                                                       |
| <b>3 star</b> | not a bad place to stay if you 're looking for a cheap place to stay .                                                                                                                                                                                                                                               |
| <b>4 star</b> | this is a great place to stay if you 're looking for a quick bite .                                                                                                                                                                                                                                                  |
| <b>5 star</b> | i love this place ! the staff is very friendly and helpful and the price is right !                                                                                                                                                                                                                                  |

Table 8: Text generated by conditioning on sentiment label.
